# Supplementary material for: Equivalence-based Security for Querying Encrypted Databases: Theory and Application to Privacy Policy Audits
Source: arXiv:1508.02448 source file (2015-08-10)
Supplement: Supplementary file 1 [file appendix.tex]

\subsection{Proof of Security of \kh (Theorem~\ref{thm:security:kh})}

The proof is in the standard model and by hybrid argument. Additionally, it depends 
on the security proof of the adjustable hash by Popa~\etal~\cite{ADJJOIN}. We proof 
that if \adv can win the \CPLAKH game with probability higher 
than $\frac{1}{2}+\pred{negl}(\param)$ then \adv can break the security  of 
adjustable hash with probability  greater than $\frac{1}{2}+\pred{negl}(\param)$. 

For contradiction, let us consider that \adv can win the \CPLAKH game with probability greater than 
$\frac{1}{2}+\pred{negl}(\param)$. Let $e\cL_0$ and $e\cL_1$ be corresponding encrypted 
logs of the plaintext logs $\cL_0$ and $\cL_1$, respectively. 
Recall that, in \kh 
an encrypted value of plaintext $v$ corresponds to a hash value, ciphertext pair (\ie, $\langle h^v, e^v\rangle$). 

We will replace some encrypted values of $e\cL_0$  with some other encrypted values to 
transform the encrypted audit log $e\cL_0$ to $e\cL_1$. If the adversary can distinguish 
$\cL_0$ and $\cL_1$ from either $e\cL_0$ or $e\cL_1$, we will show that \adv can distinguish 
 encrypted logs 
$e\cL'$ and $e\cL''$ where $e\cL''$ is obtained after a transformation 
of $e\cL'$. However, we will then show that \adv cannot distinguish $e\cL'$ and $e\cL''$ for any intermediate steps. 

Consider the first such steps of transformation. 
In each step $i >0$, we choose any cell $c$ in the intermediate log $e\cL^{(i-1)}$ (\ie, $e\cL^{(i-1)} = e\cL_0$)   
containing the encryption $\langle h^v, e^v\rangle$ such that the same value appears 
in  cell $c$ in $e\cL_0$, and replace the encryption 
with $\langle h^v, e^w\rangle$, where $w$ is the bijection image of $v$ 
in log $e\cL_1$ (\ie, $\langle -, e^w\rangle$ appears in cell $c$ in $e\cL_1$), 
to obtain the intermediate log $e\cL^i$.   
For $i > 0$, the difference between the two encrypted audit logs $e\cL^{(i-1)}$ and $e\cL^i$, 
is the cell value $\langle h^v, e^v\rangle$ is replaced with $\langle h^v, e^w\rangle$.  
We continue this until we have replaced all the ciphertexts (\eg, $e^v$) in all cells 
in $e\cL_0$ with the  ciphertexts of the corresponding cells (\eg, $e^w$)  in $e\cL_1$. 
Let us consider that after 
the final  transformation (step $n$) the log we end up with is $e\cL$. 
In $e\cL$, for each cell $l$, the hash value comes from the  cell $l$ of 
$e\cL_0$ whereas the ciphertext comes from the cell $l$ of $e\cL_1$.     

It is very clear that \adv cannot distinguish  $e\cL_0$ from $e\cL$. Because 
we use a semantically secure encryption scheme for the ciphertext portion of the 
encrypted value. Hence, if \adv could distinguish $e\cL_0$ from $e\cL$, then he would 
break semantic security of the encryption scheme. 

Now we will show some sequence of transformations to convert $e\cL$ to $e\cL_1$. 
At each step $j > n$ ($e\cL^n = e\cL$), 
we select an arbitrary column equivalence class under $\mymap^*$ and a non-constant 
plaintext value $v$ that appears in the those columns in $\cL_0$.  
We replace all hashed value of $v$ with corresponding column keys in $e\cL^{(j-1)}$ with hashed value of $w$ with appropriate keys 
where $w\in\cL_1$ is the bijection image of $v$ according to plaintext equivalence to obtain the log $e\cL^{j}$. We continue until  
all such hash values have been replaced. Then we will end up with audit log $e\cL_1$. 

If \adv can differentiate $\cL_0$ and $\cL_1$ based on $e\cL_0$ and $e\cL_1$, and as \adv cannot distinguish 
$e\cL_0$ and $e\cL$ (semantic security), then there are two consecutive transformed logs $e\cL^{(j-1)}$ and $e\cL^j$
that \adv distinguished. The only difference between these two logs is that we replaced the hash value of some $v$ with some 
keys in $e\cL^{(j-1)}$ with its bijection image $w$ with the same keys to obtain $e\cL^j$. That means there is one equivalent class of columns for which the adversary 
distinguished the two logs. 

%%%%%%%%%%%%%%%%%%%%%%%%%%%%%%%%%%%%%%%%%%%%%%%%%%%%%%%%%%%%%

%%%%%%%%%%%%%%%%%%%%%%%%%%%%%%%%%%%%%%%%%%%%%%%%%%%%%%%%%%%%%

%\subsection{Overheads of encryption on disk-backed logs}

%\begin{figure*}[t]
%\centering 
%% {
%% \renewcommand{\arraystretch}{0.001}
%%\setlength{\tabcolsep}{-23pt}
%% \setlength{\tabulinesep}{-12pt}
%\begin{tabular}{@{}cc@{}}
%%\hspace*{-0.3in}
%\includegraphics[scale=0.71]{files/hipaa-disk-time.pdf} & \includegraphics[scale=0.71]{files/glba-disk-time.pdf}
%\end{tabular}
%% }
%% \vspace*{-0.3in}
%\caption{\textbf{Experimental results for disk-backed database (HIPAA \& GLBA)}\label{fig:disk-timing}}
%\end{figure*}
